# Supplementary material for: Benchmarking Secure Sampling Protocols for Differential Privacy
Source: arXiv:2409.10667 source file (2024-11-01)
Supplement: Supplementary file 1 [file appendix.tex]

\tw{https://scholar.google.com/citations?view_op=view_citation&hl=en&user=OFBLi7gAAAAJ&sortby=pubdate&citation_for_view=OFBLi7gAAAAJ:eQOLeE2rZwMC
Free gap estimates from the exponential mechanism, sparse vector, noisy max and related algorithms
}

\section{Proof of Proposition \ref{p0} and \ref{p1}}
\label{p0p1}
We first prove that for $N\ge 2\sigma^2/t$:
\begin{equation*}
    \frac{\sum_{|n|<N} e^{-n^2/(2\sigma^2)}}{\sum_{|n|<N} e^{-|n|/t}} \ge \frac{\sum_{n\in\mathbb{Z}} e^{-n^2/2\sigma^2}}{\sum_{n\in\mathbb{Z}} e^{-|n|/t}}
\end{equation*}
Denote $a(n) \triangleq e^{-|n|/t}$ and  $b(n) \triangleq e^{-n^2/(2\sigma^2)}$, it is equivalent to proving that

\begin{equation*}
 \frac{\sum_{n\in\mathbb{Z}}b(n)}{\sum_{n\in\mathbb{Z}}a(n)}\le \frac{\sum_{|n|<N}b(n)}{\sum_{|n|<N}a(n)}
\end{equation*}
Consider the ratio between $b(n)$ and $a(n)$:
\begin{equation*}
    c(n)=\frac{b(n)}{a(n)}=\exp(\frac{-(|n|-\sigma^2/t)^2 }{2\sigma^2}+\frac{\sigma^2}{2t^2})
\end{equation*}
then we have for $m\ge 2\sigma^2/t$, $\underset{|n|\ge m}{\max} c(n) = \underset{|n|\le m}{\min} c(n)= c(m)$.
Therefore, for  $N\ge 2\sigma^2/t$, we have
\begin{equation*}
     \frac{\sum_{|n|<N}b(n)}{\sum_{|n|<N}a(n)} \ge \underset{|n| < N}{\min}c(n) \ge \underset{|n| \le N}{\min}c(n) = c(N)
\end{equation*}

\begin{equation*}
     \frac{\sum_{|n|\ge N}b(n)}{\sum_{|n|\ge N}a(n)} \le \underset{|n| \ge N}{\max}c(n)  = c(N)
\end{equation*}
which follows $\frac{\sum_{|n|<N}b(n)}{\sum_{|n|<N}a(n)}\ge \frac{\sum_{|n|\ge N}b(n)}{\sum_{|n|\ge N}a(n)}$, thus

\begin{equation*}
     \frac{\sum_{n\in\mathbb{Z}}b(n)}{\sum_{n\in\mathbb{Z}}a(n)} = \frac{\sum_{|n|<N}b(n)+\sum_{|n|\ge N}b(n)}{\sum_{|n|<N}a(n)+\sum_{|n|\ge N}a(n)} \le \frac{\sum_{|n|<N}b(n)}{\sum_{|n|<N}a(n)}
\end{equation*}

%\begin{equation*}
Now we consider to estimate $p_*$, denote:
\begin{equation*}
    I(t) \triangleq \sum_{n\in \mathbb{Z}} e^{-|n|/t}, J(\sigma) \triangleq \sum_{n\in\mathbb{Z}} e^{-n^2/(2\sigma^2)}
\end{equation*}
\begin{equation*}
S(t,\sigma) \triangleq e^{-\sigma^2/(2t^2)}
\end{equation*}
then we have, for $N\ge 2\sigma^2/t$
\begin{equation*}
\begin{aligned}
p_* &= \frac{\sum_{|n|<N} e^{-n^2/(2\sigma^2)}}{\sum_{|n|<N} e^{-|n|/t}} \cdot e^{-\sigma^2/(2t^2)} \\ &\ge\frac{\sum_{n\in\mathbb{Z}}e^{-n^2/(2\sigma^2)}}{\sum_{n\in\mathbb{Z}}e^{-|n|/t}} \cdot e^{-\sigma^2/(2t^2)} = \frac{J(\sigma)}{I(t)} \cdot S(t,\sigma) \\
\end{aligned}
\end{equation*}
based on the inequalities $J(\sigma)\ge\max(1,\sqrt{2\pi}\sigma)$, we get:
\begin{equation}
\label{pp}
p_*\ge \frac{S(t,\sigma)}{I(t)}\cdot \max(1,\sqrt{2\pi}\sigma)
\end{equation}

For $\sigma \ge 1, t=\sigma^2 / \lfloor \sigma \rceil$ and $N\ge 2\lfloor \sigma \rceil$, in this case $N\ge 2\sigma^2/t$ is satisfied, based on \eqref{pp} we have:
% according to (\ref{ee}) we get the lower-bound of $p_*$ that:
\begin{equation*}
p_* \ge \frac{S(\sigma^2 / \lfloor \sigma \rceil,\sigma)}{I(\sigma^2 / \lfloor \sigma \rceil)}\cdot \sqrt{2\pi}\sigma \triangleq g_0(\sigma)
\end{equation*}
since $g_0(\sigma)$ is convex in $(n-1/2, n+1/2]$ for $n\in\mathbb{N}^+$, the possible minimum points are $1$, $1.5^-$, $1.5^+$, $2.5^-$, $2.5^+$, $3.5^-$, $3.5^+...$ . We construct two auxiliary functions:
\begin{equation*}
\begin{aligned}
    g_1(\sigma) \triangleq=& \frac{S(\sigma^2 / (\sigma -1/2),\sigma)}{I(\sigma^2 / (\sigma-1/2))}\cdot \sqrt{2\pi}\sigma\\
    g_2(\sigma) \triangleq=& \frac{S(\sigma^2 / (\sigma +1/2),\sigma)}{I(\sigma^2 / (\sigma+1/2))}\cdot \sqrt{2\pi}\sigma\\
\end{aligned}
\end{equation*}
which satisfy 
\begin{equation*}
    g_0((n+1/2)^-) = g_1(n+1/2) \quad g_0((n+1/2)^+) = g_2(n+1/2)
\end{equation*}
for $n\in\mathbb{N}^+$. Notice that both $g_1(\sigma)$ and $g_2(\sigma)$ are monotonically increasing when $\sigma \ge 1$, which means that  
\begin{equation*}
\begin{aligned}
    g_0(1.5^-) < g_0(2.5^-) < g_0(3.5^-) < ... \\
    g_0(1.5^+) < g_0(2.5^+) < g_0(3.5^+) < ...
\end{aligned}
\end{equation*}
Thus the possible minimum points are $1, 1.5^-$ and $1.5^+$. We calculate and compare these three values and get the lower bound of $p_*$
\begin{equation*}
\label{e0}
    p_* \ge \min_{\sigma\ge1} g_0(\sigma) = \min(g_0(1), g_0(1.5^-), g_0(1.5^+)) > 0.64
\end{equation*}
Therefore we have $p_* > 0.64$ when $\sigma \ge 1$ and $N\ge 2\lfloor \sigma \rceil$.
\vspace{3pt}

For $\sigma\in (0,1)$ and $t=\sigma^2  \lceil 1/\sigma \rceil$, in this case $N\ge 2\sigma^2/t$ is always satisfied. We consider $\sigma\in(0,1)$ in three intervals $[\frac{1}{\sqrt{2\pi}}, 1)$, $[\frac14, \frac{1}{\sqrt{2\pi}}]$ and $(0, \frac14)$ respectively.

\noindent For $\sigma \in [\frac{1}{\sqrt{2\pi}}, 1)$, based on \eqref{pp} we have:
\begin{equation*}
p_* \ge \frac{S(\sigma^2  \lceil 1/\sigma \rceil,\sigma)}{I(\sigma^2  \lceil 1/\sigma \rceil)}\cdot \sqrt{2\pi}\sigma \triangleq h_0(\sigma)
\end{equation*}
since $h_0(\sigma)$ is convex in $[\frac{1}{\sqrt{2\pi}},\frac12)$ and $[\frac12, 1)$, the possible minimum points are $\frac{1}{\sqrt{2\pi}}^+, \frac12^-, \frac12^+$ and $1^-$. We calculate and compare these four values and get:
\begin{equation}
\label{e1}
\begin{aligned}
    &p_* \ge \min_{\sigma \in [\frac1{\sqrt{2\pi}},1)} h_0(\sigma) \\
    &= \min(h_0(\frac1{\sqrt{2\pi}}^+),h_0(\frac12^-),h_0(\frac12^+),h_0(1^-)) > 0.54
\end{aligned}
\end{equation}
For $\sigma \in [\frac14, \frac1{\sqrt{2\pi}})$, based on \eqref{pp} we have:
\begin{equation*}
p_* \ge \frac{S(\sigma^2  \lceil 1/\sigma \rceil,\sigma)}{I(\sigma^2  \lceil 1/\sigma \rceil)}\triangleq h_2(\sigma)
\end{equation*}
Since $h_1(\sigma)$ is convex in $[\frac13, \frac1{\sqrt{2\pi}})$ and $[\frac14, \frac13)$, the possible minimum points are $\frac1{\sqrt{2\pi}}^-, \frac13^-, \frac13^+$ and $\frac14^+$, we calculate and compare this four values and get:
\begin{equation}
\label{e2}
\begin{aligned}
    &p_* \ge \min_{\sigma \in [\frac14, \frac1{\sqrt{2\pi}})} h_1(\sigma) \\ &= \min(h_1(\frac1{\sqrt{2\pi}}^-), h_1(\frac13^-), h_1(\frac13^+), h_1(\frac14^+)) > 0.54
\end{aligned}
\end{equation}
For $\sigma \in (0, \frac14)$, based on \eqref{pp} we have:
\begin{equation*}
p_* \ge \frac{S(\sigma^2  \lceil 1/\sigma \rceil,\sigma)}{I(\sigma^2  \lceil 1/\sigma \rceil)}
\end{equation*}
notice that $S(t,\sigma)$ is monotonically increasing with $t$, and $I(t)$ is monotonically decreasing with $t$, then:
\begin{equation*}
p_* \ge \frac{S(\sigma^2  \lceil 1/\sigma \rceil,\sigma)}{I(\sigma^2  \lceil 1/\sigma \rceil)} \ge \frac{S(\sigma^2 (1/\sigma),\sigma)}{I(\sigma^2 (1/\sigma + 1))} = \frac{S(\sigma,\sigma)}{I(\sigma^2 + \sigma)}\triangleq h_2(\sigma)
\end{equation*}
since $h_2(\sigma)$ is monotonically decreasing when $0 < \sigma < 1$, we have:
\begin{equation}
\label{e3}
    p_* \ge \min_{\sigma \in (0, \frac14)} h_2(\sigma) = h_2(\frac14^-) > 0.55
\end{equation}
According to \eqref{e1}, ~\eqref{e2}, ~\eqref{e3}, we have $p_* > 0.54$ when $\sigma \in (0,1)$.

\section{Proof of Theorem \ref{ssd}} 
\label{proofmulti}

According to Section \ref{dgaudp}, we obtain that
\begin{equation}
\label{w1}
    \mathrm{SD}(\mathcal{N}_{\mathbb{Z}}^n(\sigma), \mathcal{N}_{\mathbb{Z}, N}^n(\sigma)) \le 2n e^{-\frac{N^2}{2\sigma^2}}
\end{equation}

First, we consider the statistical distance between $\mathcal{G}_{2^\kappa}$ and the output distribution $\mathcal{G}'$  of Algorithm \ref{tgeo}. Notice that the sample of $\mathcal{G}_{2^\kappa}$ can be seen as $\kappa$ independent Bernoulli samples, with each sample having at most $2^{-\mu}$ statistical distance based on Algorithm \ref{tgeo}. Therefore, we have:
\begin{equation}
\label{sdg}
    \mathrm{SD}(\mathcal{G}'_{2^\kappa}, \mathcal{G}_{2^\kappa}) \le \kappa \cdot 2^{-\mu}
\end{equation}

Denote $N=2^\kappa+1$,  we consider statistical distance between $\mathcal{L}_{\mathbb{Z},N}$ and the output  distribution  $\mathcal{L}'$ of Algorithm \ref{algo:dlap}. Notice that we use a Bernoulli sample to determine whether to output $0$ or other values, then we have:
\begin{equation*}
    f_{\mathcal{L}'}(0) = f_{\mathcal{L}_{\mathbb{Z},N}}(0) + \delta_d \\
\end{equation*}
for some $|\delta_d| \le 2^{-\mu}$ and $f_{\mathcal{L}_{\mathbb{Z},N}}(0) + \delta_d \in [0,1]$. Then for $x\neq 0$, we have
\begin{equation*}
    f_{\mathcal{L}'}(x) = \frac12 (1 - f_{\mathcal{L}_{\mathbb{Z},N}}(0) - \delta_d) \cdot  f_{\mathcal{G}_{2^\kappa}}(|x|-1) 
\end{equation*}
According to \eqref{sdg}, we have: 
\begin{equation*}
    f_{\mathcal{G}'}(x)=f_{\mathcal{G}_{2^\kappa}}(x)+\delta_g(x)
\end{equation*}
with $\sum_x |\delta_g(x)| \le 2\kappa \cdot 2^{-\mu}$. Then
\begin{equation}
\label{sdl}
\begin{aligned}
    &\mathrm{SD}(\mathcal{L}_{\mathbb{Z},N}, \mathcal{L}') = \frac 12 \sum_x | f_\mathcal{L'}(x) - f_\mathcal{L}(x)  | \\
    & = \frac 12 ( | f_{\mathcal{L}'}(0) - f_{\mathcal{L}_{\mathbb{Z},N}}(0)  | + \sum_{x\neq 0} | f_{\mathcal{L}'}(x) - f_{\mathcal{L}_{\mathbb{Z},N}}(x)  | ) \\
    &\le  \frac 12  \left( |\delta_d| + (1-f_{\mathcal{L}_{\mathbb{Z},N}}(0)-\delta_b) \sum_{x} |\delta_g(x)| + |\delta_d|  \sum_{x}  f_{\mathcal{G}_{2^\kappa}}(x) \right) \\
    &\le  \frac12 (2 |\delta_d| + \sum_{x} |\delta_g(x)|) \le (\kappa + 1) \cdot 2^{-\mu}
\end{aligned}
\end{equation}

Next we consider the statistical distance between $\mathcal{A}=\mathcal{B}(\exp(-u/r))$ and the output distribution $\mathcal{A}'$ of the Algorithm \ref{expber}. Notice the $\mathcal{A}$ is sampled by combined $l$ independent Bernoulli samples from $\mathcal{A}_i=\mathcal{B}(\exp(-2^i/r))$, such that
\begin{equation*}
    f_{A}(1) = \prod_{i=0}^{l-1} \left(1-u_i f_{\mathcal{A}_i}(0)\right) = \prod_{i=0}^{l-1} (1-u_ip_i)
\end{equation*}
Here $u=\sum_{i=0}^{l-1}u_i2^i$ with $u_i\in\{0,1\}$. Then, we have
\begin{equation*}
    f_{\mathcal{A}'}(1)= \prod_{i=0}^{l-1} (1 - u_i (p_i + \delta_i)) 
\end{equation*}
for each $|\delta_i| \le 2^{-\mu}$ and $p_i+\delta_i \in [0,1]$. Denote $d_i=1-u_ip_i$, then $d_i-u_i\delta_1 \in [0,1]$ and $d_i\in[0,1]$. It leads to
\begin{equation}
\label{sda}
\begin{aligned}
    &\mathrm{SD}(\mathcal{A}', \mathcal{A}) =  | f_{\mathcal{A}'}(1) - f_{\mathcal{A}}(1) |   \\
    &= \left| \prod_{i=0}^{l-1} (d_i - u_i \delta_i) - \prod_{i=0}^{l-1} d_i  \right| \le \sum_{i=0}^{l-1} u_i| \delta_i| \le l \cdot 2^{-\mu}
\end{aligned}
\end{equation}

Finally, we focus on rejection sampling $\mathcal{N}_{\mathbb{Z}, N}$. Actually, we use $\mathcal{L}'$ as proposal distribution and sample accept bit from $\mathcal{A}'$. According to \eqref{sdl}, \eqref{sda}, we have
\begin{equation*}
\begin{aligned}
    &f_{\mathcal{L}'}(x)=f_{\mathcal{L}_{\mathbb{Z},N}}(x) + \delta_l(x) \\
   &f_{\mathcal{A}'}(1;x) = f_{\mathcal{A}}(1;x) + \delta_a = \frac{f_{\mathcal{N}_{\mathbb{Z},N}}(x) }{M\cdot f_{\mathcal{L}_{\mathbb{Z},N}}(x) } + \delta_a 
\end{aligned}
\end{equation*}
with $\ \sum_x |\delta_l(x)| \le 2(\kappa + 1)\cdot 2^{-\mu}$ and $\delta_a \le l\cdot 2^{-\mu}$. The actual average accept probability $p'$ is:
\begin{equation*}
\begin{aligned}
    p'&=\sum_x f_{\mathcal{L}'}(x) \cdot  f_{\mathcal{A}'}(1;x) \\
        &= \sum_x(f_{\mathcal{L}_{\mathbb{Z},N}}(x) + \delta_l(x)) \cdot (\frac{f_{\mathcal{N}_{\mathbb{Z},N}}(x) }{M\cdot f_{\mathcal{L}_{\mathbb{Z},N}}(x) } + \delta_a ) \\
        &= \frac1M +  \sum_x \delta_n(x) = p_* + \sum_x \delta_n(x)
\end{aligned}
\end{equation*}
Here $\delta_n(x)=\delta_l(x) \cdot f_{\mathcal{A}'}(1;x) + f_{\mathcal{L}_{\mathbb{Z},N}}(x) \cdot \delta_a$, which satisfies
\begin{equation*}
    \sum_x |\delta_n(x)|\le \sum_x |\delta_l(x)| + |\delta_a| \le (2\kappa + l + 2)\cdot 2^{-\mu}
\end{equation*}
Therefore, the lower bound of $p'$ is
\begin{equation*}
    p'\ge p_* - \sum_x |\delta_n(x)|\ge  p_* -(2\kappa+l+2)\cdot 2^{-\mu} = p'_*
\end{equation*}
And the actual target distribution $\mathcal{W}$ becomes
\begin{equation*}
    f_{\mathcal{W}}(x) = \frac{f_{\mathcal{L}'}(x) \cdot f_{\mathcal{A}'}(1;x)}{p'} =\frac{ p_*  f_{\mathcal{N}_{\mathbb{Z}, N}}(x) + \delta_n(x)}{ p_* + \sum_t \delta_n(t) }
\end{equation*}
The statistical distance between the $\mathcal{W}$ and $\mathcal{N}_{\mathbb{Z}, N}$ is
\begin{equation*}
\begin{aligned}
    &\mathrm{SD}(\mathcal{W}, \mathcal{N}_{\mathbb{Z}, N}) = \frac12 \sum_x \left| f_{\mathcal{W}}(x) - f_{\mathcal{N}_{\mathbb{Z}, N}}(x) \right|  \\
    &= \frac12 \sum_x  \left|\frac{ p_*  f_{\mathcal{N}_{\mathbb{Z}, N}}(x) + \delta_n(x)}{ p_* + \sum_t \delta_n(t) } -  f_{\mathcal{N}_{\mathbb{Z}, N}}(x) \right| \\
    &= \frac {\sum_x | \delta_n(x) - \sum_t \delta_n(t) f_{\mathcal{N}_{\mathbb{Z}, N}}(x) |}{2( p_* + \sum_t \delta_n(t))} \\
    &\le  \frac {\sum_x |\delta_n(x)| + \sum_t |\delta_n(t)| \cdot \sum_x f_{\mathcal{N}_{\mathbb{Z}, N}}(x) }{2( p_* + \sum_t \delta_n(t))} \\
    &\le \frac {(2\kappa + l + 2)\cdot 2^{-\mu}}{ p'} \le \frac {(2\kappa + l + 2)\cdot 2^{-\mu}}{p_*'}
\end{aligned}
\end{equation*}
If follows that
\begin{equation}
\label{w2}
\begin{aligned}
    \mathrm{SD}(\mathcal{W}^{n}, \mathcal{N}^n_{\mathbb{Z}, N}) &\le \frac {n}{p_*'} \cdot(2\kappa + l + 2)\cdot 2^{-\mu}\\
\end{aligned}
\end{equation}
Denote $\mathcal{V}$ as the output distribution of Algorithm \ref{alg:dgau}, which uses $m$ trials to generate $n$ independent samples in $\mathcal{W}$. Denote $E$ as the event that $m$ trials fail to generate $n$ samples, s.t.
\begin{equation*}
\begin{aligned}
    \Pr{E} &= \Pr{X < n\mid X \sim \mathbf{Bin}(m,p')} \\
         &\le \Pr{X < n\mid X \sim \mathbf{Bin}(m,p_*')}
\end{aligned}
\end{equation*}
Here $\mathcal{I}$ is the binomial distribution. Then we have
\begin{equation*}
    f_\mathcal{V}(x) = \Pr{\neg E} \cdot f_{\mathcal{W}^n}(x) + \Pr{E} \cdot e(x)
\end{equation*}
Here $e(x)$ is the probability of output $x$ when $E$ happens. The statistical distance between $\mathcal{W}^n$ and $\mathcal{V}$ is:
\begin{equation}
\label{w3}
\begin{aligned}
    &\mathrm{SD}(\mathcal{V}, \mathcal{W}^n) = \frac 12 \left|   f_\mathcal{V}(x) - f_{\mathcal{W}^n}(x) \right| \\
    &= \frac 12 \sum_x \left| \Pr{E} (f_{\mathcal{W}^n}(x) - e(x)) \right| \\
    &\le \frac12\cdot \Pr{E} \left(\sum_x f_{\mathcal{W}^n}(x) + \sum_x e(x)\right) = \Pr{E}
\end{aligned}
\end{equation}

Combine \eqref{w1},~\eqref{w2},~\eqref{w3}, according to the triangle inequality, we obtain that
\begin{equation*}
\begin{aligned}
    \mathrm{SD}(\mathcal{N}^n_\mathbb{Z}, \mathcal{V}) &\le   \mathrm{SD}(\mathcal{N}^n_\mathbb{Z}, \mathcal{N}^n_{\mathbb{Z},N})  \\ &+\mathrm{SD}(\mathcal{N}^n_{\mathbb{Z},N}, \mathcal{W}^n) +
    \mathrm{SD}(\mathcal{N}^n_{\mathcal{W}^n}, \mathcal{V}) \\
    &= \delta_t + \delta_b + \delta_r
\end{aligned}
\end{equation*}
Here
\begin{equation*}
\begin{aligned}
\delta_t &= 2ne^{-\frac{N^2}{2\sigma^2}} \\
\delta_b  &= \frac{n}{p_*} \cdot(2\kappa + l + 2)\cdot 2^{-\mu}\\
\delta_r &=\Pr{X < n\mid X \sim \mathcal{I}(m,p_*')}
\end{aligned}
\end{equation*}
with $p_*'=  p_* -(2\kappa+l+2)\cdot 2^{-\mu}$

%%% Local Variables:
%%% mode: latex
%%% TeX-master: "main"
%%% End:

\begin{table}[h]
\centering
\caption{Some MPC subprotocols mentioned in this paper. }
\label{table:notation}
\begin{tabular}{cc}
\toprule
MPC subprotocol & Output / Functionality \\
\midrule
$\textbf{EQ}(\langle a \rangle ,\langle b \rangle)$  & If $a=b$, $\langle 1 \rangle$, else $\langle 0 \rangle$ \\
$\textbf{LE}(\langle a \rangle ,\langle b \rangle)$ & If $a\leq b$, $\langle 1 \rangle$, else $\langle 0 \rangle$ \\
$\textbf{SUB}(\langle a \rangle ,\langle b \rangle)$  & $\langle a - b \rangle$ \\
$\textbf{ABS}(\langle a \rangle)$  & $\langle |a| \rangle$ \\
$\textbf{XOR}(\langle a \rangle ,\langle b \rangle)$ & $\langle a \oplus b \rangle$ \\
$\textbf{MUX}(\langle a \rangle ,\langle b \rangle, \langle c \rangle)$ & If $a=1$, $\langle b \rangle$, else $\langle c \rangle$ \\
$\textbf{UBIT}()$ \cite{wei2023securely} & A uniform random bit $\langle b \rangle$\\
$\textbf{SORT}(\langle A \rangle) $ \cite{keller2020mp} & Securely sort list $\langle A \rangle$ \\
$\textbf{CPUSH}(\langle a \rangle, \langle b \rangle, \textbf{s})$ \cite{champion2019securely} & If $a = 1$, push bit $b$ into stack $\textbf{s}$ \\
$\textbf{RPOP}(\textbf{s})$ \cite{champion2019securely} & $\langle a \rangle $ on top of stack $\textbf{s}$ \\
$\textbf{CRESET}(\langle a \rangle, \textbf{s})$ \cite{champion2019securely} & If $a = 1$, reset stack $\textbf{s}$ \\
$\textbf{PURGE}(\textbf{s})$ \cite{champion2019securely} & $\langle X \rangle$ list of all bits in stack $\textbf{s}$ \\
\bottomrule
\end{tabular}
\end{table}
